# Supplementary material for: Expanding Boundaries: Cross-Media Routing for Seamless Underwater and Aerial Communication
Source: arXiv:2307.12643 source file (2023-07-24)
Supplement: Supplementary file 1 [file appendix.tex]

\section{Appendix A}
From here we avoid to use the index $k$ for simplicity,
As $A^{\dagger}$ is a $3*L$ dimension matrix and we know that our desired component of $X$ lies in $\hat{X}$. Now let $\hat{A^{\dagger}}=A_{2*L}^{\dagger}$, then (7) can also be written as
\begin{align}
\hat{X}=\hat{A^{\dagger}}b
\end{align}
Or more precisely
\begin{align}
\hat{X}=\underbrace{\hat{A^{\dagger}}\begin{bmatrix}
      {d_1}^2-x_1^2-y_1^2 \\
    .   \\
     .\\
       {d_L}^2-x_L^2-y_L^2   
  \end{bmatrix}}_{True \ Co-ordinates} + \underbrace{2\hat{A^{\dagger}}\begin{bmatrix}
      n_1d_1\\
    .   \\
     .\\
       n_Ld_L   
  \end{bmatrix}}_{Noise}
\end{align} 
